# Supplementary material for: Your Smart Home Can't Keep a Secret: Towards Automated Fingerprinting of IoT Traffic with Neural Networks
Source: arXiv:1909.00104 source file (2019-08-31)
Supplement: Supplementary file 1 [file appendix_test.tex]

\section{Appendix}
